# Supplementary material for: On Robustness of Prompt-based Semantic Parsing with Large Pre-trained Language Model: An Empirical Study on Codex
Source: arXiv:2301.12868 source file (2026-11-13)
Supplement: Supplementary file 1 [file appendix_rq_3.tex]

\begin{table*}[]
    \small
    \centering
    \begin{tabular}{ccc|cccccc|c}
    \hline
         Dataset & $n$-shot & Context & AdvLogProb & LMF & ED & TF-IDF & PPL. Asc & PPL. Desc & Random*\\\hline
        \multirow{15}{*}{AdvGeoQuery} & \multirow{3}{*}{10} & \{Std\} & 59.65 & 64.37 & 66.10 & 68.05 & 53.77 & 40.28 & 56.80\\
        & & $\Delta$ \{Adv\} & +5.15 & +6.29 & +5.37 & +7.97 &+2.93  & +1.24 & +4.19\\
        & & $\Delta$ \{Std + Adv\} & +8.53 &+7.51 &+5.95 & +8.70 &+1.61 & +1.34 & +3.92\\\cline{2-10}
        & \multirow{3}{*}{20}  & \{Std\} &  60.13 & 65.63 & 69.87 & 70.22 & 57.65 & 42.94 & 57.50\\
        & & $\Delta$ \{Adv\}& +7.54 & +4.30 & +6.91 & +6.39 &+2.95  & +1.56 & +3.84\\
        & & $\Delta$ \{Std + Adv\} & +9.69 & +7.95 & +7.42 & +6.83 & +3.79 & +1.43 & +5.52\\\cline{2-10}
        & \multirow{3}{*}{30} & \{Std\} & 64.19 & 67.59 & 71.25 & 74.84 & 59.38 & 41.04 & 59.49\\
        & & $\Delta$ \{Adv\} & +9.26 & +6.35 & +6.21 & +5.11 & +5.70 & +0.89 & +4.94\\
        & & $\Delta$ \{Std + Adv\} & +9.63 & +7.84 & +8.30 & +5.14 & +4.95 & +0.27 & +3.35\\\cline{2-10}
        & \multirow{3}{*}{40} & \{Std\} & 66.75 & 69.35 & 75.20 & 76.36 & 61.32 & 44.53 & 64.42\\
        & & $\Delta$ \{Adv\} &+9.30 & +6.57 & +5.54 & +8.73 & +2.28 & -0.03 & +6.50\\
        & & $\Delta$ \{Std + Adv\} & +8.94 & +7.88 & +4.39 & +8.76 & +3.14 & +0.42 & +6.23\\\cline{2-10}
        & \multirow{3}{*}{50} & \{Std\} & 69.80 & 68.93 & 74.41 & 77.74 & 62.11 & 45.71 & 66.58\\
        & & $\Delta$ \{Adv\} & +8.04 & +10.55 & +5.41 & +9.48 & +2.40 & -1.88 & +8.73\\
        & & $\Delta$ \{Std + Adv\} & +10.59 & +11.95 & +7.14 & +10.61 & +1.91 & +0.42 & +9.53\\\hline\hline
        \multirow{9}{*}{AdvScholar} & \multirow{3}{*}{3} & \{Std\} & 8.00 & 8.27 & 8.69 & 9.38 & 4.39 & 1.66 & 7.71\\\
        & & $\Delta$ \{Adv\} & +1.74 & +1.05 & +0.89 & +1.10 & +0.82 & +0.78 & +0.37\\
        & & $\Delta$ \{Std + Adv\} & +1.01 & +1.35 & +1.95 & +1.99 & +0.31 & +0.18 & +1.66\\\cline{2-10}
        & \multirow{3}{*}{5} & \{Std\} & 17.67  & 20.93 & 23.00 & 28.81 & 16.14 & 4.68 & 16.27\\
        & & $\Delta$ \{Adv\} & +3.46 & +4.88 & +3.38 & +1.42 & +2.78 & +0.14 & +2.13\\
        & & $\Delta$ \{Std + Adv\} & +2.77 & +4.90 & +5.58 & +2.22 & +1.69 & +1.63 & +2.68\\\cline{2-10}
        & \multirow{3}{*}{10} & \{Std\} & 28.55  & 29.81 & 30.28 & 31.44 & 22.25 & 7.47 & 25.35\\
        & & $\Delta$ \{Adv\} & +6.68 & +5.97 & +6.53 & +7.56 & +5.27 & +0.51 & +8.70\\
        & & $\Delta$ \{Std + Adv\} & +7.72 & +8.49 & +6.89 & +9.21 & +6.60 & +0.12 & +8.33\\\hline
    \end{tabular}
    \caption{}
    \label{tab:my_label}
\end{table*}

\begin{table*}[]
    \small
    \centering
    \begin{tabular}{cc|ccccccc}
    \hline
         Dataset & LC. Metric & AdvLogProb & LMF & ED & TF-IDF & PPL. Asc & PPL. Desc & Random*\\\hline
        \multirow{3}{*}{GeoQuery} & TTR & 7.68 & 7.24 & 8.47 & 10.26 & 5.94 & 3.22 & 6.44\\
        & Yule's I & 68.55 & 64.37 & 69.59 & 71.49 & 62.94 & 43.41 & 58.14\\
        & MTLD & 12.44 & 12.19 & 13.37 & 15.58 & 11.32 & 8.16 & 10.41\\\hline
        \multirow{3}{*}{Scholar} & TTR & 28.18 & 29.91 & 31.40 & 33.11 & 21.15 & 14.17 & 25.67\\
        & Yule's I & 198.15 & 207.11 & 223.76 & 262.36 & 177.37 & 102.17 & 193.31\\
        & MTLD & 15.68 & 15.63 & 16.34 & 19.49 & 11.94 & 13.12 & 14.36\\\hline
    \end{tabular}
    \caption{\{Std\}, 50-shot of GeoQuery, 10-shot of Scholar; TTR, multiplied by 100; Yule's I, multiplied by 100;}
    \label{tab:my_label}
\end{table*}
